# Supplementary material for: Heralded-Multiplexed High-Efficiency Cascaded Source of Dual-Rail Polarization-Entangled Photon Pairs using Spontaneous Parametric Down Conversion
Source: arXiv:2107.14360 source file (2021-07-29)
Supplement: Supplementary file 6 [file appendix_completepattern.tex]

\begin{supertabular}[htbp]
    \centering
    \resizebox{0.625\textwidth}{!}{\begin{tabular}{c c c c c c}
        \toprule
        Source 1 & Source 2 & Coeff. & Output & Click Pattern & Heralded Output\\
       \midrule
       $\ket{0,0,0,0}$ & $\ket{0,0,0,0}$ & 1 & $\ket{0,0,0,0;0,0,0,0}$ & (0,0,0,0) & $\ket{0,0;0,0}$\\
        \midrule \midrule
         $\ket{0,0,0,0}$ & $\ket{1,0,0,1}$ &  $1/\sqrt{2}$  & $\ket{0,0,0,0;1,0,0,1}$ & (0,0,1,0) & $\ket{0,0;0,1}$\\
         {} & {} &  $1/\sqrt{2}$  & $\ket{0,0,1,0;0,0,0,1}$ & (1,0,0,0) & {}\\
        \midrule
        $\ket{0,0,0,0}$ & $\ket{0,1,1,0}$ & $1/\sqrt{2}$ & $\ket{0,0,0,0;0,1,1,0}$ & (0,0,0,1)& $\ket{0,0;1,0}$\\
         {} & {} & $1/\sqrt{2}$ & $\ket{0,0,0,1;0,0,1,0}$ & (0,1,0,0)& {}\\
        \midrule
        $\ket{1,0,0,1}$ & $\ket{0,0,0,0}$ &  $1/\sqrt{2}$ & $\ket{1,0,0,1;0,0,0,0}$ & (0,1,0,0) & $ \ket{1,0;0,0} $\\
         {} & {} &  $-1/\sqrt{2}$ & $\ket{1,0,0,0;0,1,0,0}$ & (0,0,0,1) & {}\\
         \midrule
        $\ket{0,1,1,0}$ & $\ket{0,0,0,0}$ &  $1/\sqrt{2}$ & $\ket{0,1,1,0;0,0,0,0}$ & (1,0,0,0) & $ \ket{0,1,0,0} $\\
         {} & {} &  $-1/\sqrt{2}$ & $\ket{0,1,0,0;1,0,0,0}$ & (0,0,1,0) & {}\\
        \midrule \midrule
        $\ket{1,0,0,1}$ & $\ket{1,0,0,1}$ & 1/2 & $\ket{1,0,0,1;1,0,0,1}$ & {(0,1,1,0)} & $ \ket{1,0;0,1} $\\
         {} & {} & $-1/2$ & $\ket{1,0,1,1;0,0,0,1}$ & (1,1,0,0)& $ {} $\\
         {} & {} & $1/2$ & $\ket{1,0,0,0;1,1,0,1}$ & (0,0,1,1)& $ {} $\\
         {} & {} & $-1/2$ & $\ket{1,0,1,0;0,1,0,1}$ & {(1,0,0,1)}& $ {} $\\
        \midrule
         $\ket{0,1,1,0}$ & $\ket{0,1,1,0}$ & 1/2 & $\ket{0,1,1,0;0,1,1,0}$ & {(1,0,0,1)} & $ \ket{0,1;1,0} $\\
         {} & {} & $-1/2$ & $\ket{0,1,1,1;0,0,1,0}$ & (1,1,0,0)& $ {} $\\
         {} & {} & $1/2$ & $\ket{0,1,0,0;1,1,1,0}$ & (0,0,1,1)& $ {} $\\
         {} & {} & $-1/2$ & $\ket{0,1,1,0;0,1,1,0}$ & {(0,1,1,0)} & $ {} $\\
        \midrule
        $\ket{1,0,0,1}$ & $\ket{0,1,1,0}$ & $-1/\sqrt{2}$ & $\ket{1,0,0,2;0,0,1,0}$ & (0,2,0,0)& $\ket{1,0,1,0}$\\
         {} & {} & $1/\sqrt{2}$ & $\ket{1,0,0,0;0,2,1,0}$ & (0,0,0,2)& {}\\
         \midrule
        $\ket{0,1,1,0}$ & $\ket{1,0,0,1}$ & $-1/\sqrt{2}$ & $\ket{0,1,2,0;0,0,0,1}$ & (2,0,0,0) & $\ket{0,1,0,1}$\\
         {} & {} & $1/\sqrt{2}$ & $\ket{0,1,0,0;2,0,0,1}$ & (0,0,2,0) & {}\\
        \midrule\midrule
        $\ket{0,0,0,0}$ & $\ket{1,1,1,1}$ & $1/2$ & $\ket{0,0,0,0;1,1,1,1}$ & (0,0,1,1) & $ \ket{0,0;1,1} $\\
        {} & {} & $-1/2$ & $\ket{0,0,1,0;0,1,1,1}$ & {(1,0,0,1)}& $ {} $\\
        {} & {} & $-1/2$ & $\ket{0,0,0,1;1,0,1,1}$ & {(0,1,1,0)}& $ {} $\\
        {} & {} & $1/2$ & $\ket{0,0,1,1;0,0,1,1}$ & {(1,1,0,0)}& $ {} $\\
        \midrule
        $\ket{1,1,1,1}$ & $\ket{0,0,0,0}$ & $1/2$ & $\ket{1,1,1,1;0,0,0,0}$ & (1,1,0,0) & $ \ket{1,1;0,0} $\\
        {} & {} & $1/2$ & $\ket{1,1,0,1;1,0,0,0}$ & {(0,1,1,0)}& $ {} $\\
        {} & {} & $1/2$ & $\ket{1,1,1,0;0,1,0,0}$ & {(1,0,0,1)}& $ {} $\\
        {} & {} & $1/2$ & $\ket{1,1,0,0;1,1,0,0}$ & {(0,0,1,1)}& $ {} $\\
        \midrule\midrule
        $\ket{0,0,0,0}$ & $\ket{2,0,0,2}$ & 1/2 & $\ket{0,0,0,0;2,0,0,2}$ & (0,0,2,0) & $ \ket{0,0;0,2} $\\
        {} & {} & $-1/\sqrt{2}$ & $\ket{0,0,1,0;1,0,0,2}$ & {(1,0,1,0)}& $ {} $\\
        {} & {} & $1/2$ & $\ket{0,0,2,0;0,0,0,2}$ & {(2,0,0,0)}& $ {} $\\
        \midrule
        $\ket{0,0,0,0}$ & $\ket{0,2,2,0}$ & 1/2 & $\ket{0,0,0,0;0,2,2,0}$ & (0,0,0,2) & $ \ket{0,0;2,0} $\\
        {} & {} & $-1/\sqrt{2}$ & $\ket{0,0,0,1;0,1,2,0}$ & {(0,1,0,1)}& $ {} $\\
        {} & {} & $1/2$ & $\ket{0,0,0,2;0,0,2,0}$ & {(0,2,0,0)}& $ {} $\\
        \midrule
        $\ket{2,0,0,2}$ & $\ket{0,0,0,0}$ & 1/2 & $\ket{2,0,0,2;0,0,0,0}$ & (0,2,0,0) & $ \ket{2,0;0,0} $\\
        {} & {} & $1/\sqrt{2}$ & $\ket{2,0,0,1;0,1,0,0}$ & {(0,1,0,1)}& $ {} $\\
        {} & {} & $1/2$ & $\ket{2,0,0,0;0,2,0,0}$ & {(0,0,0,2)}& $ {} $\\
        \midrule
        $\ket{0,2,2,0}$ & $\ket{0,0,0,0}$ & 1/2 & $\ket{0,2,2,0;0,0,0,0}$ & (2,0,0,0) & $ \ket{0,2;0,0} $\\
        {} & {} & $1/\sqrt{2}$ & $\ket{0,2,1,0;1,0,0,0}$ & {(1,0,1,0)}& $ {} $\\
        {} & {} & $1/2$ & $\ket{0,2,0,0;2,0,0,0}$ & {(0,0,2,0)}& $ {} $\\
        \midrule
        \bottomrule
    \end{tabular}}
\caption{The complete table considering all input term combinations and detection patterns are given here.}
\label{tab:complete}
\end{supertabular}
